# Supplementary material for: Upside/Downside statistical mechanics of nonequilibrium Brownian motion. I. Distributions, moments, and correlation functions of a free particle
Source: arXiv:1908.00503 ancillary file (2019-08-01)
Supplement: Supplementary file 1 [file Supplement.pdf]

# Supplemental Material for "Upside/Downside statistical mechanics of nonequilibrium Brownian motion. I. Distributions, moments, and correlation functions of a free particle"

Galen T. Craven[1] and Abraham Nitzan[1,2]

[1]Department of Chemistry, University of Pennsylvania, Philadelphia, PA 19104, USA

[2]School of Chemistry, Tel Aviv University, Tel Aviv 69978, Israel

## I. DERIVATIONS OF STEADY-STATE RESTRICTED TRANSPORT PROPERTIES

In this section of the Supplemental Material, explicit forms are given for the one- and two-time integrals used to evaluate the restricted transition probabilities, probability densities, moments, and correlation functions discussed in the main text. Except where noted, evaluating these integrals, which are combinations of exponential functions (Gaussian functions) and error functions, is straightforward and can be accomplished using known methods and integral tables [1–4].

### A. One-time Restricted Properties

There are two types of integrals that appear in the derivations of the one-time upside/downside restricted properties. The first type:

$$I_{\uparrow}^{(1)}(t) \equiv \int_{\mathbb{R}^2} v^k \rho_0(\bar{v})\rho(v\,t\,|\,\bar{v}\,0)\Theta\big(E(v) - E^{\ddagger}\big)dv\,d\bar{v}, \tag{S1}$$

$$I_{\downarrow}^{(1)}(t) \equiv \int_{\mathbb{R}^2} v^k \rho_0(\bar{v})\rho(v\,t\,|\,\bar{v}\,0)\Theta\big(E^{\ddagger} - E(v)\big)dv\,d\bar{v}, \tag{S2}$$

where $k$ is a nonnegative integer, is used to evaluate the restricted upside/downside probabilities and velocity moments, and the second type:

$$I_{\uparrow}^{(2)}(v,t) \equiv \int_{\mathbb{R}} \rho_0(\bar{v})\rho(v\,t\,|\,\bar{v}\,0)\Theta\big(E(v) - E^{\ddagger}\big)d\bar{v}, \tag{S3}$$

$$I_{\downarrow}^{(2)}(v,t) \equiv \int_{\mathbb{R}} \rho_0(\bar{v})\rho(v\,t\,|\,\bar{v}\,0)\Theta\big(E^{\ddagger} - E(v)\big)d\bar{v}, \tag{S4}$$

arises in calculations of the restricted probability densities.

*$E(t)$ compared to $E(0)$*— In the case $\rho_0 = \rho^{(\mathrm{ss})}$ and $E^{\ddagger} = E(0)$, the $I^{(1)}$ integrals for upside and

downside processes take the respective forms:

$$I_{\uparrow}^{(1)}(t) \propto \int_{-\infty}^{\infty} \int_{-|v|}^{|v|} v^k \exp\left[-\frac{m\bar{v}^2}{2k_{\mathrm{B}}T}\right] \exp\left[-\left(\frac{v-\bar{v}e^{-\gamma t}}{\sqrt{2\sigma_v^2(t)}}\right)^2\right] d\bar{v}\, dv, \tag{S5}$$

$$I_{\downarrow}^{(1)}(t) \propto \int_{-\infty}^{\infty} \int_{-|\bar{v}|}^{|\bar{v}|} v^k \exp\left[-\frac{m\bar{v}^2}{2k_{\mathrm{B}}T}\right] \exp\left[-\left(\frac{v-\bar{v}e^{-\gamma t}}{\sqrt{2\sigma_v^2(t)}}\right)^2\right] dv\, d\bar{v}, \tag{S6}$$

where the constraints imposed by Heaviside functions in Eqs. (S1) and (S2) have been written explicitly in the bounds of integration. Note that for upside processes $\bar{v}$ is integrated over the region $(-|v|, |v|)$ and for downside processes $v$ is integrated over the region $(-|\bar{v}|, |\bar{v}|)$. Also note that the time-dependent coefficients of proportionality which appear explicitly in the main text have been omitted for notational convenience. The $I^{(2)}$ integrals are

$$I_{\uparrow}^{(2)}(v,t) \propto \int_{-|v|}^{|v|} \exp\left[-\frac{m\bar{v}^2}{2k_{\mathrm{B}}T}\right] \exp\left[-\left(\frac{v-\bar{v}e^{-\gamma t}}{\sqrt{2\sigma_v^2(t)}}\right)^2\right] d\bar{v}, \tag{S7}$$

$$\begin{aligned} I_{\downarrow}^{(2)}(v,t) \propto & \int_{-\infty}^{-|v|} \exp\left[-\frac{m\bar{v}^2}{2k_{\mathrm{B}}T}\right] \exp\left[-\left(\frac{v-\bar{v}e^{-\gamma t}}{\sqrt{2\sigma_v^2(t)}}\right)^2\right] d\bar{v} \\ & + \int_{|v|}^{\infty} \exp\left[-\frac{m\bar{v}^2}{2k_{\mathrm{B}}T}\right] \exp\left[-\left(\frac{v-\bar{v}e^{-\gamma t}}{\sqrt{2\sigma_v^2(t)}}\right)^2\right] d\bar{v}. \end{aligned} \tag{S8}$$

Standard methods can be used to evaluate the $I^{(1)}$ and $I^{(2)}$ integrals in terms of exponential and error functions.

*$E(t)$ relative to $\langle E \rangle$*— For $\rho_0 = \rho^{(\mathrm{ss})}$ and $E^{\ddagger} = \langle E \rangle$, the $I^{(1)}$ integrals are

$$I_{\uparrow}^{(1)}(t) \propto \int_{-\infty}^{\infty} \int_{-\sqrt{\langle v^2 \rangle}}^{\sqrt{\langle v^2 \rangle}} v^k \exp\left[-\frac{m\bar{v}^2}{2k_{\mathrm{B}}T}\right] \exp\left[-\left(\frac{v-\bar{v}e^{-\gamma t}}{\sqrt{2\sigma_v^2(t)}}\right)^2\right] d\bar{v}\, dv, \tag{S9}$$

$$I_{\downarrow}^{(1)}(t) \propto \int_{-\infty}^{\infty} \int_{-\sqrt{\langle v^2 \rangle}}^{\sqrt{\langle v^2 \rangle}} v^k \exp\left[-\frac{m\bar{v}^2}{2k_{\mathrm{B}}T}\right] \exp\left[-\left(\frac{v-\bar{v}e^{-\gamma t}}{\sqrt{2\sigma_v^2(t)}}\right)^2\right] dv\, d\bar{v}. \tag{S10}$$

Note that the order of integration has been interchanged in the upside and downside expressions and that the bounds of integration in both integrals do not depend on $v$ or $\bar{v}$ because $\sqrt{\langle v^2 \rangle} = \sqrt{k_{\mathrm{B}}T/m}$. The second $I^{(2)}$-type integrals are used to evaluate the restricted probability densities. For upside

and downside processes these integrals take the respective forms:

$$I_{\uparrow}^{(2)}(v,t) \propto \int_{-\sqrt{\langle v^2\rangle}}^{\sqrt{\langle v^2\rangle}} \exp\left[-\frac{m\bar{v}^2}{2k_{\mathrm{B}}T}\right] \exp\left[-\left(\frac{v-\bar{v}e^{-\gamma t}}{\sqrt{2\sigma_v^2(t)}}\right)^2\right] d\bar{v}, \tag{S11}$$

$$I_{\downarrow}^{(2)}(v,t) \propto \int_{-\infty}^{-\sqrt{\langle v^2\rangle}} \exp\left[-\frac{m\bar{v}^2}{2k_{\mathrm{B}}T}\right] \exp\left[-\left(\frac{v-\bar{v}e^{-\gamma t}}{\sqrt{2\sigma_v^2(t)}}\right)^2\right] d\bar{v} + \int_{\sqrt{\langle v^2\rangle}}^{\infty} \exp\left[-\frac{m\bar{v}^2}{2k_{\mathrm{B}}T}\right] \exp\left[-\left(\frac{v-\bar{v}e^{-\gamma t}}{\sqrt{2\sigma_v^2(t)}}\right)^2\right] d\bar{v}, \tag{S12}$$

which can be evaluated in a straightforward manner.

### B. Two-time Restricted Properties

There are two main types of integrals that appear in the derivations of the upside/downside two-time restricted properties. The first type:

$$I_{\uparrow}^{(1)}(t,t') \equiv \int_{\mathbb{R}^3} v^k v'^l \rho_0(\bar{v})\rho(v\,t\,|\,v'\,t')\rho(v'\,t'\,|\,\bar{v}\,0)\Theta\big(E(v)-E^{\ddagger}\big)dv\,dv'd\bar{v}, \tag{S13}$$

$$I_{\downarrow}^{(1)}(t,t') \equiv \int_{\mathbb{R}^3} v^k v'^l \rho_0(\bar{v})\rho(v\,t\,|\,v'\,t')\rho(v'\,t'\,|\,\bar{v}\,0)\Theta\big(E^{\ddagger}-E(v)\big)dv\,dv'd\bar{v}, \tag{S14}$$

where $k$ and $l$ are nonnegative integers, are used to evaluate the restricted velocity and energy moments and velocity correlation functions. The second type:

$$I_{\uparrow}^{(2)}(v',t,t') \equiv \int_{\mathbb{R}^2} \rho_0(\bar{v})\rho(v\,t\,|\,v'\,t')\rho(v'\,t'\,|\,\bar{v}\,0)\Theta\big(E(v)-E^{\ddagger}\big)dv\,d\bar{v}, \tag{S15}$$

$$I_{\downarrow}^{(2)}(v',t,t') \equiv \int_{\mathbb{R}^2} \rho_0(\bar{v})\rho(v\,t\,|\,v'\,t')\rho(v'\,t'\,|\,\bar{v}\,0)\Theta\big(E^{\ddagger}-E(v)\big)dv\,d\bar{v}, \tag{S16}$$

are used to evaluate the upside/downside probability densities at time $t' < t$.

*$E(t)$ compared to $E(0)$*— In the case with $\rho_0 = \rho^{(\mathrm{ss})}$ and $E^{\ddagger} = E(0)$, the $I^{(1)}$ integrals are

$$I_{\uparrow}^{(1)}(t,t') \propto \int_{-\infty}^{\infty}\int_{-\infty}^{\infty}\int_{-|v|}^{|v|} v^k v'^l \exp\left[-\frac{m\bar{v}^2}{2k_{\mathrm{B}}T}\right] \times \exp\left[-\left(\frac{v-v'e^{-\gamma(t-t')}}{\sqrt{2\sigma_v^2(t-t')}}\right)^2\right] \exp\left[-\left(\frac{v'-\bar{v}e^{-\gamma t'}}{\sqrt{2\sigma_v^2(t')}}\right)^2\right] d\bar{v}\,dv'dv, \tag{S17}$$

$$I_{\downarrow}^{(1)}(t,t') \propto \int_{-\infty}^{\infty}\int_{-\infty}^{\infty}\int_{-|\bar{v}|}^{|\bar{v}|} v^k v'^l \exp\left[-\frac{m\bar{v}^2}{2k_{\mathrm{B}}T}\right] \times \exp\left[-\left(\frac{v-v'e^{-\gamma(t-t')}}{\sqrt{2\sigma_v^2(t-t')}}\right)^2\right] \exp\left[-\left(\frac{v'-\bar{v}e^{-\gamma t'}}{\sqrt{2\sigma_v^2(t')}}\right)^2\right] dv\,dv'd\bar{v}. \tag{S18}$$

The $I^{(2)}$ integrals are

$$I_{\uparrow}^{(2)}(v',t,t') \propto \int_{-\infty}^{\infty}\int_{-|v|}^{|v|} \exp\left[-\frac{m\bar{v}^2}{2k_{\mathrm{B}}T}\right] \times \exp\left[-\left(\frac{v-v'e^{-\gamma(t-t')}}{\sqrt{2\sigma_v^2(t-t')}}\right)^2\right] \exp\left[-\left(\frac{v'-\bar{v}e^{-\gamma t'}}{\sqrt{2\sigma_v^2(t')}}\right)^2\right] d\bar{v}\, dv, \tag{S19}$$

$$I_{\downarrow}^{(2)}(v',t,t') \propto \int_{-\infty}^{\infty}\int_{-|\bar{v}|}^{|\bar{v}|} \exp\left[-\frac{m\bar{v}^2}{2k_{\mathrm{B}}T}\right] \times \exp\left[-\left(\frac{v-v'e^{-\gamma(t-t')}}{\sqrt{2\sigma_v^2(t-t')}}\right)^2\right] \exp\left[-\left(\frac{v'-\bar{v}e^{-\gamma t'}}{\sqrt{2\sigma_v^2(t')}}\right)^2\right] dv\, d\bar{v}, \tag{S20}$$

which can be written as combinations of the two general integral forms $I^{(2a)}$ and $I^{(2b)}$:

$$I_{\uparrow}^{(2a)}(v',t,t') = \int_{-\infty}^{\infty} \exp\left[-(\alpha_1\bar{v}+\alpha_2)^2\right] \operatorname{erf}\left[\alpha_3\bar{v}+\alpha_4\right] d\bar{v} = \frac{\sqrt{\pi}}{2}\operatorname{erf}\left[\frac{\alpha_1\alpha_4-\alpha_2\alpha_3}{\sqrt{\alpha_1^2+\alpha_3^3}}\right], \tag{S21}$$

$$I_{\downarrow}^{(2a)}(v',t,t') = \int_{-\infty}^{\infty} \exp\left[-(\alpha_1'v+\alpha_2')^2\right] \operatorname{erf}\left[\alpha_3'v+\alpha_4'\right] dv = \frac{\sqrt{\pi}}{2}\operatorname{erf}\left[\frac{\alpha_1'\alpha_4'-\alpha_2'\alpha_3'}{\sqrt{\alpha_1'^2+\alpha_3'^2}}\right], \tag{S22}$$

and

$$I_{\uparrow}^{(2b)}(v',t,t') = \int_{0}^{\infty} \exp\left[-(\alpha_1\bar{v}+\alpha_2)^2\right] \operatorname{erf}\left[\alpha_3\bar{v}+\alpha_4\right] d\bar{v}, \tag{S23}$$

$$I_{\downarrow}^{(2b)}(v',t,t') = \int_{0}^{\infty} \exp\left[-(\alpha_1'v+\alpha_2')^2\right] \operatorname{erf}\left[\alpha_3'v+\alpha_4'\right] dv, \tag{S24}$$

where $\alpha_j$ and $\alpha_j'$ are functions that may depend on $v'$, $t'$, and/or $t$. Integrals of type $I^{(1)}$ and $I^{(2a)}$ have closed-form expressions and can be evaluated using typical methods. The $I^{(2b)}$ integrals, however, cannot be expressed in closed-form but can be evaluated analytically by representing the error and exponential functions in series form [3, 4].

*$E(t)$ relative to $\langle E\rangle$*— For $\rho_0 = \rho^{(\mathrm{ss})}$ and $E^{\ddagger} = \langle E\rangle$, the upside and downside $I^{(1)}$ integrals are

$$I_{\uparrow}^{(1)}(t,t') \propto \int_{-\infty}^{\infty}\int_{-\infty}^{\infty}\int_{-\sqrt{\langle v^2\rangle}}^{\sqrt{\langle v^2\rangle}} v^k v'^l \exp\left[-\frac{m\bar{v}^2}{2k_{\mathrm{B}}T}\right] \times \exp\left[-\left(\frac{v-v'e^{-\gamma(t-t')}}{\sqrt{2\sigma_v^2(t-t')}}\right)^2\right] \exp\left[-\left(\frac{v'-\bar{v}e^{-\gamma t'}}{\sqrt{2\sigma_v^2(t')}}\right)^2\right] d\bar{v}\, dv' dv, \tag{S25}$$

$$I_{\downarrow}^{(1)}(t,t') \propto \int_{-\infty}^{\infty}\int_{-\infty}^{\infty}\int_{-\sqrt{\langle v^2\rangle}}^{\sqrt{\langle v^2\rangle}} v^k v'^l \exp\left[-\frac{m\bar{v}^2}{2k_{\mathrm{B}}T}\right] \times \exp\left[-\left(\frac{v-v'e^{-\gamma(t-t')}}{\sqrt{2\sigma_v^2(t-t')}}\right)^2\right] \exp\left[-\left(\frac{v'-\bar{v}e^{-\gamma t'}}{\sqrt{2\sigma_v^2(t')}}\right)^2\right] dv\, dv' d\bar{v}, \tag{S26}$$

and the upside and downside $I^{(2)}$ integrals are:

$$I_{\uparrow}^{(2)}(v', t, t') \propto \int_{-\infty}^{\infty} \int_{-\sqrt{\langle v^2 \rangle}}^{\sqrt{\langle v^2 \rangle}} \exp\left[-\frac{m\bar{v}^2}{2k_{\mathrm{B}}T}\right] \times \exp\left[-\left(\frac{v - v' e^{-\gamma(t-t')}}{\sqrt{2\sigma_v^2(t-t')}}\right)^2\right] \exp\left[-\left(\frac{v' - \bar{v}e^{-\gamma t'}}{\sqrt{2\sigma_v^2(t')}}\right)^2\right] d\bar{v}\, dv, \tag{S27}$$

$$I_{\downarrow}^{(2)}(v', t, t') \propto \int_{-\infty}^{\infty} \int_{-\sqrt{\langle v^2 \rangle}}^{\sqrt{\langle v^2 \rangle}} \exp\left[-\frac{m\bar{v}^2}{2k_{\mathrm{B}}T}\right] \times \exp\left[-\left(\frac{v - v' e^{-\gamma(t-t')}}{\sqrt{2\sigma_v^2(t-t')}}\right)^2\right] \exp\left[-\left(\frac{v' - \bar{v}e^{-\gamma t'}}{\sqrt{2\sigma_v^2(t')}}\right)^2\right] dv\, d\bar{v}. \tag{S28}$$

Both of these integral types can be evaluated in a straightforward manner.

## II. RESTRICTED TRANSPORT PROPERTIES FOR $\rho_0 = \delta(v - v_0)$ AND $E^{\ddagger} = E(0)$

### A. One-time Restricted Transition Probabilities and Probability Densities

For a free Brownian particle with velocity distribution $\rho_0 = \delta(v - v_0)$ at time $t = 0$, in the limit $t \to \infty$ the process approaches a steady state (ss) and the restricted probabilities $p_{\uparrow}^{(\mathrm{ss})}$ and $p_{\downarrow}^{(\mathrm{ss})}$ that a process with initial energy $E(0) = \frac{1}{2}mv_0^2$ is in higher energy state (upside process $\uparrow$) or lower energy state (downside process $\downarrow$) are

$$p_{\uparrow}^{(\mathrm{ss})}[E(0)] = \int_{-\infty}^{\infty} \int_{E(0)}^{\infty} \rho^{(\mathrm{ss})}(v)\delta(E(v) - \epsilon)\, dv\, d\epsilon = \mathrm{erfc}\left(\sqrt{\beta E(0)}\right), \tag{S29}$$

and

$$p_{\downarrow}^{(\mathrm{ss})}[E(0)] = \int_{-\infty}^{\infty} \int_{0}^{E(0)} \rho^{(\mathrm{ss})}(v)\delta(E(v) - \epsilon)\, dv\, d\epsilon = \mathrm{erf}\left(\sqrt{\beta E(0)}\right), \tag{S30}$$

respectively. These probabilities can also be evaluated directly in energy space:

$$p_{\uparrow}^{(\mathrm{ss})}[E(0)] = \frac{\displaystyle\int_{E(0)}^{\infty} g(\epsilon)e^{-\beta\epsilon}\, d\epsilon}{\displaystyle\int_{0}^{\infty} g(\epsilon)e^{-\beta\epsilon}\, d\epsilon} = \mathrm{erfc}\left(\sqrt{\beta E(0)}\right), \tag{S31}$$

$$p_{\downarrow}^{(\mathrm{ss})}[E(0)] = \frac{\displaystyle\int_{0}^{E(0)} g(\epsilon)e^{-\beta\epsilon}\, d\epsilon}{\displaystyle\int_{0}^{\infty} g(\epsilon)e^{-\beta\epsilon}\, d\epsilon} = \mathrm{erf}\left(\sqrt{\beta E(0)}\right), \tag{S32}$$

where $g(\epsilon)$ is the density of states at energy $\epsilon$ that can be obtained through an inverse Laplace transform of the canonical partition function $Z^{(\mathrm{ss})}$:

$$g(\epsilon) = \mathcal{L}^{-1}\left\{Z^{(\mathrm{ss})}(\beta)\right\} \propto \sqrt{\frac{1}{\epsilon}}. \tag{S33}$$

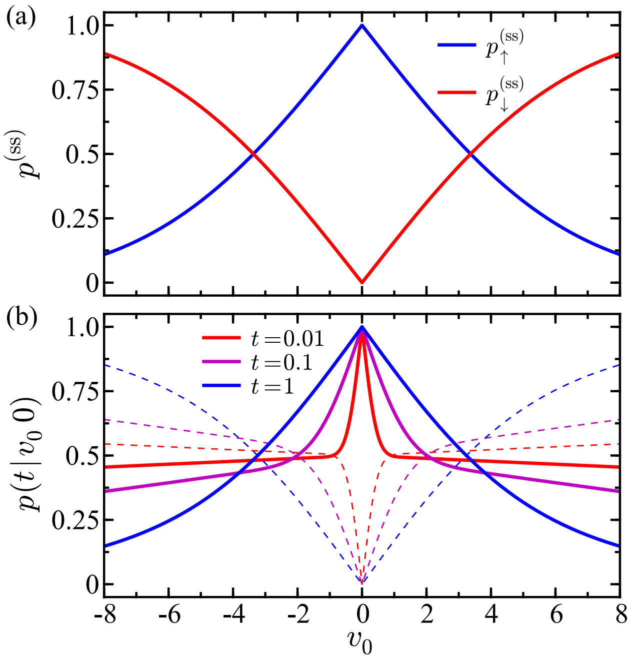


FIG. S1. (a) Steady-state probability that a process with initial velocity $v_0$ is an upside process (blue) or downside process (red). (b) Probability that a process with initial velocity $v_0$ is an upside process (solid) or downside process (dashed) for various values of $t$. In both panels the threshold energy is $E^\ddagger = E(0)$. Parameters in this and all other figures are $\gamma = 1$ ($\gamma_1 = 1/4$, $\gamma_2 = 3/4$), $m = 1$, and $T = 1$ ($T_1 = 4/5$, $T_2 = 16/15$) which are given in reduced units with characteristic dimensions: length $\widetilde{\sigma} = 1\,\text{Å}$, time $\widetilde{\tau} = 1\,\text{ps}$, mass $\widetilde{m} = 10\,m_u$, and temperature $\widetilde{T} = 300\,\text{K}$.

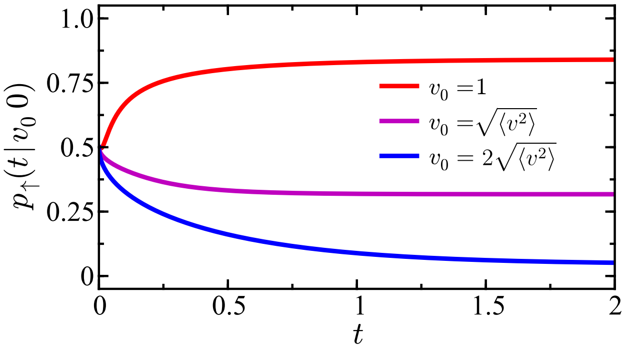


FIG. S2. Time-dependence of the upside probability for various values of $v_0$. In both panels the threshold energy is $E^\ddagger = E(0)$

The functional forms of $p_\uparrow^{(ss)}$ and $p_\uparrow^{(ss)}$ are shown in Fig S1(a) with respect to variation of $v_0$. For $v_0 = 0$, the process must increase in energy and consequently $p_\uparrow^{(ss)} = 1$ and $p_\downarrow^{(ss)} = 0$. In the opposite limit as $|v_0| \to \infty$, the upside probability $p_\uparrow^{(ss)} \to 0$ and the downside probability $p_\downarrow^{(ss)} \to 1$.

For initial distribution $\rho_0 = \delta(v - v_0)$ and energy threshold $E^\ddagger = E(0)$, the restricted proba-

bilities that a process with initial velocity $v_0$ has increased or decreased in energy at time $t$, are, respectively,

$$\begin{aligned} p_{\uparrow}\Big(t \,\big|\, E(t) > E(0), v_0\, 0\Big) &\equiv p_{\uparrow}(t \,|\, v_0\, 0) \\ &= \int_{\mathbb{R}} \rho(v\, t \,|\, v_0\, 0)\Theta\big(v^2 - v_0^2\big)\, dv \\ &= 1 - \Phi\big(|v_0|, v_0; t\big) + \Phi\big(-|v_0|, v_0; t\big), \end{aligned} \tag{S34}$$

and

$$\begin{aligned} p_{\downarrow}\Big(t \,\big|\, E(t) < E(0), v_0\, 0\Big) &\equiv p_{\downarrow}(t \,|\, v_0\, 0) \\ &= \int_{\mathbb{R}} \rho(v\, t \,|\, v_0\, 0)\Theta\big(v_0^2 - v^2\big)\, dv \\ &= \Phi\big(|v_0|, v_0; t\big) - \Phi\big(-|v_0|, v_0; t\big), \end{aligned} \tag{S35}$$

where

$$\begin{aligned} \Phi(\alpha, v_0; t) &= \int_{-\infty}^{\alpha} \rho(v\, t \,|\, v_0\, 0)\, dv \\ &= \frac{1}{2}\,\mathrm{erfc}\left[\frac{v_0 e^{-\gamma t} - \alpha}{\sqrt{2\sigma_v^2(t)}}\right], \end{aligned} \tag{S36}$$

is the time-dependent cumulative distribution function. Shown in Fig. S1(b) are the upside $p_{\uparrow}$ and downside $p_{\downarrow}$ transition probabilities as a function of $v_0$ for different values of $t$. As in the steady-state limit, for $v_0 = 0$ the process must increase in energy and $p_{\uparrow} = 1$. In the limit $t \to \infty$, the time-dependent restricted transition probabilities approach the respective steady-state probabilities. In the opposite limit:

$$\lim_{t\to 0} p_{\uparrow}\Big(t \,\big|\, E(t) > E(0), v_0\, 0\Big) = \begin{cases} 1, & v_0 = 0 \\ 1/2, & v_0 \neq 0 \end{cases}, \tag{S37}$$

$$\lim_{t\to 0} p_{\downarrow}\Big(t \,\big|\, E(t) < E(0), v_0\, 0\Big) = \begin{cases} 0, & v_0 = 0 \\ 1/2, & v_0 \neq 0 \end{cases}, \tag{S38}$$

which show that a process has equal probability to increase or decrease in energy as $t \to 0$, except for a system prepared in the lowest energy state. Thus, both $p_{\uparrow}$ and $p_{\downarrow}$ have a singularity at $v_0 = 0$. The formation of this singularity can be observed in Fig. S1(b) by comparing the probability curves at descending values of $t$. Shown in Fig. S2 is the time-dependence of the upside probability $p_{\uparrow}(t)$ for various values of $v_0$. At $t = 0$, $p_{\uparrow} = 1/2$ for all values of $v_0 \neq 0$. Note that in the long-time limit the restricted probabilities are highly dependent on the specific value of $v_0$, which can also

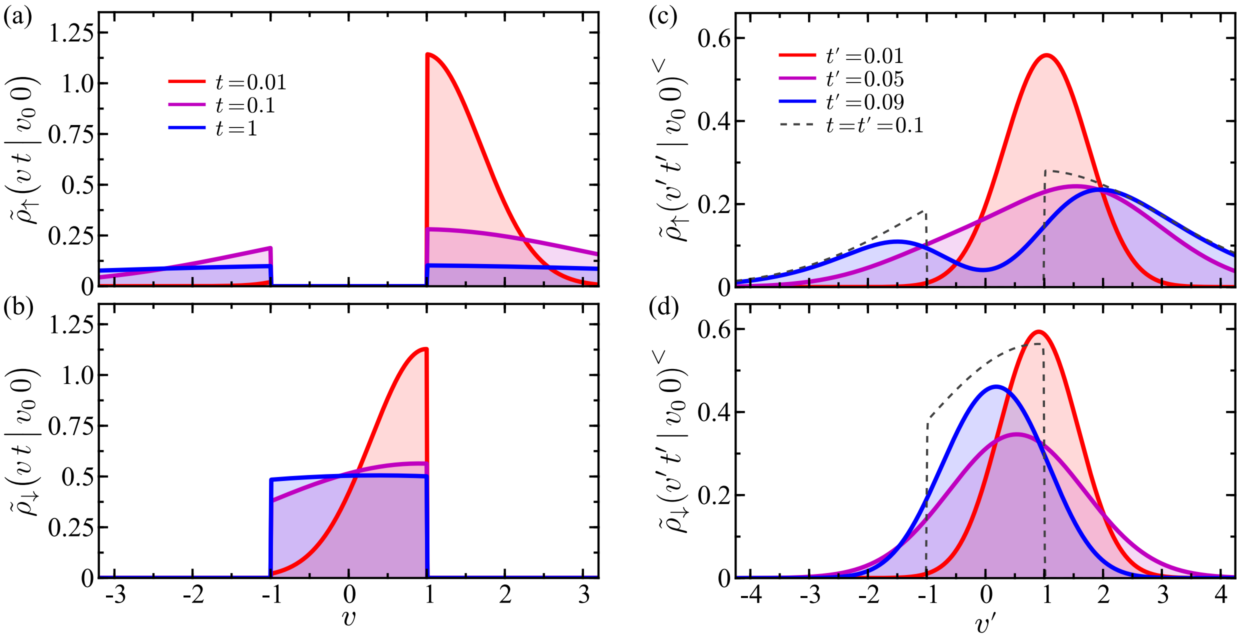


FIG. S3. Restricted upside and downside probability density for $\rho_0 = \delta(v - v_0)$ with $v_0 = 1$ as (a)-(b) functions of $v$ for different values of $t$ marked in the legend of (a), and (c)-(d) functions of $v'$ for different values of $t' < t$ marked in the legend of (c). In panels (c)-(d) the upside/downside constraint is imposed at $t = 0.1$ and the dashed curves correspond to the respective densities at the $t' = t$ limit. In all panels the threshold energy is $E^{\ddagger} = E(0)$.

be observed in Fig. S1(a), and that in the specific case of $v_0 = \sqrt{\langle v^2 \rangle} \approx 5$ which implies $E_0 = \langle E \rangle$, starting with an initial energy equal to the average energy leads to time-dependent evolution in $p_{\uparrow}$.

For threshold $E^{\ddagger} = E(0)$ and an ensemble with initial distribution $\rho_0 = \delta(v - v_0)$ the restricted probability densities are, respectively:

$$\tilde{\rho}_{\uparrow}\big(v\,t\,|\,v_0\,0\big) = \frac{\rho(v\,t\,|\,v_0\,0)\Theta\big(v^2 - v_0^2\big)}{1 - \Phi\big(|v_0|, v_0; t\big) + \Phi\big(-|v_0|, v_0; t\big)}, \tag{S39}$$

$$\tilde{\rho}_{\downarrow}\big(v\,t\,|\,v_0\,0\big) = \frac{\rho(v\,t\,|\,v_0\,0)\Theta\big(v_0^2 - v^2\big)}{\Phi\big(|v_0|, v_0; t\big) - \Phi\big(-|v_0|, v_0; t\big)}, \tag{S40}$$

where the denominators normalize the density over the respective restricted space. The functional forms of the restricted densities (S39) and (S40) are shown in Fig. S3(a)-(b) as a function of $v$. Note that the upside density $\tilde{\rho}_{\uparrow}$ is nonzero on the discontinuous interval $(-\infty, -|v_0|) \cup (|v_0|, \infty)$ and the downside density $\tilde{\rho}_{\downarrow}$ is nonzero on the continuous interval $(-|v_0|, |v_0|)$.

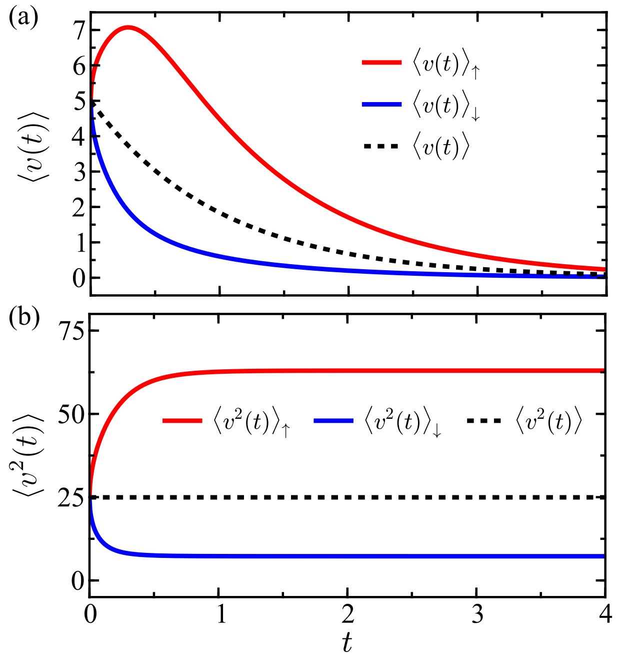


FIG. S4. Velocity moments (a) $\langle v(t)\rangle$ and (b) $\langle v^2(t)\rangle$ as a function of $t$ for restricted (solid) and unrestricted (dashed) transport and an initial distribution $\delta(v-v_0)$ with $v_0=\sqrt{\langle v^2\rangle}$. In both panels the threshold energy is $E^\ddagger = E(0)$.

### B. One-time Restricted Velocity Moments

For $E^\ddagger = E(0)$, the time-dependent upside restricted density $\tilde{\rho}_\uparrow\big(v\,t\,\big|\,v_0\,0\big)$ and the time-dependent downside restricted density $\tilde{\rho}_\uparrow\big(v\,t\,\big|\,v_0\,0\big)$ which correspond to an initial $\delta$-distribution in $v$: $\rho_0=\delta(v-v_0)$, are given by Eqs. (S39) and (S40), respectively. From the general expressions for the $k$th restricted moments given in the main text, we obtain the first restricted moments of the velocity:

$$\Big\langle v\big(t\,\big|\,E(t)>E(0),v_0\,0\big)\Big\rangle_\uparrow = \big\langle v(t)\big\rangle + \sigma_v^2(t)\left[\frac{\rho\big(|v_0|\,t\,\big|\,v_0\,0\big)-\rho\big(-|v_0|\,t\,\big|\,v_0\,0\big)}{1-\Phi\big(|v_0|,v_0;t\big)+\Phi\big(-|v_0|,v_0;t\big)}\right], \tag{S41}$$

$$\Big\langle v\big(t\,\big|\,E(t)<E(0),v_0\,0\big)\Big\rangle_\downarrow = \big\langle v(t)\big\rangle - \sigma_v^2(t)\left[\frac{\rho\big(|v_0|\,t\,\big|\,v_0\,0\big)-\rho\big(-|v_0|\,t\,\big|\,v_0\,0\big)}{\Phi\big(|v_0|,v_0;t\big)-\Phi\big(-|v_0|,v_0;t\big)}\right], \tag{S42}$$

which are shown in Fig. S4(a). Observe that the derivatives with respect to time of the upside and downside moments can have opposite signs, and thus one moment can be increasing while the other is decreasing, or vice versa — the specific behavior will depend on the value of $v_0$. In the limit $t\to\infty$, both restricted moments decay to zero.

The second restricted velocity moments are:

$$\begin{aligned}\Big\langle v^2\big(t\,\big|\,E(t)>E(0),v_0\,0\big)\Big\rangle_{\uparrow} &= \sigma_v^2(t)+\big\langle v(t)\big\rangle^2\\ &+\sigma_v^2(t)\left[\frac{\big(\langle v(t)\rangle+|v_0|\big)\rho\big(|v_0|\,t\,\big|\,v_0\,0\big)}{1-\Phi\big(|v_0|,v_0;t\big)+\Phi\big(-|v_0|,v_0;t\big)}\right]\\ &-\sigma_v^2(t)\left[\frac{\big(\langle v(t)\rangle-|v_0|\big)\,\rho\big(-|v_0|\,t\,\big|\,v_0\,0\big)}{1-\Phi\big(|v_0|,v_0;t\big)+\Phi\big(-|v_0|,v_0;t\big)}\right], \qquad \text{(S43)}\\ \Big\langle v^2\big(t\,\big|\,E(t)<E(0),v_0\,0\big)\Big\rangle_{\downarrow} &= \sigma_v^2(t)+\big\langle v(t)\big\rangle^2\\ &-\sigma_v^2(t)\left[\frac{\big(\langle v(t)\rangle+|v_0|\big)\,\rho\big(|v_0|\,t\,\big|\,v_0\,0\big)}{\Phi\big(|v_0|,v_0;t\big)-\Phi\big(-|v_0|,v_0;t\big)}\right]\\ &+\sigma_v^2(t)\left[\frac{\big(\langle v(t)\rangle-|v_0|\big)\,\rho\big(-|v_0|\,t\,\big|\,v_0\,0\big)}{\Phi\big(|v_0|,v_0;t\big)-\Phi\big(-|v_0|,v_0;t\big)}\right], \qquad \text{(S44)}\end{aligned}$$

which are shown in Fig. S4(b) as a function of $t$. Both moments decay from $\big\langle v^2(0)\big\rangle_{\uparrow}=\big\langle v^2(0)\big\rangle_{\downarrow}=v_0^2$ to an asymptotic value as $t\to\infty$.

### C. Two-time Restricted Probability Densities

For energy threshold $E^{\ddagger}=E(0)$ and initial distribution $\delta(v-v_0)$, the restricted probability densities at time $t'<t$ given that the process is upside/downside at time $t$ are:

$$\tilde{\rho}_{\uparrow}\Big(v'\,t'<t\,\big|\,E(t)>E(0),v_0\,0\Big)^{<}=\rho\big(v'\,t'\,|\,v_0\,0\big)\left[\frac{1-\Phi\big(|v_0|,v';t-t'\big)+\Phi\big(-|v_0|,v';t-t'\big)}{1-\Phi\big(|v_0|,v_0;t\big)+\Phi\big(-|v_0|,v_0;t\big)}\right], \qquad \text{(S45)}$$

$$\tilde{\rho}_{\downarrow}\Big(v'\,t'<t\,\big|\,E(t)<E(0),v_0\,0\Big)^{<}=\rho\big(v'\,t'\,|\,v_0\,0\big)\left[\frac{\Phi\big(|v_0|,v';t-t'\big)-\Phi\big(-|v_0|,v';t-t'\big)}{\Phi\big(|v_0|,v_0;t\big)-\Phi\big(-|v_0|,v_0;t\big)}\right]. \qquad \text{(S46)}$$

These restricted probability densities are shown in Figs. S3(c)-(d) as a function of $v'$ for various values of $t'<t$. In this specific case, for small values of $t'\ll t$ the upside and downside densities have similar shapes and are centered about $v'\approx v_0$. This behavior is a direct consequence of the short-time evolution from the initial $\delta$-distribution. As $t'$ is increased, the upside density becomes bimodal while the downside density takes an approximately Gaussian shape with time-varying mean and variance.

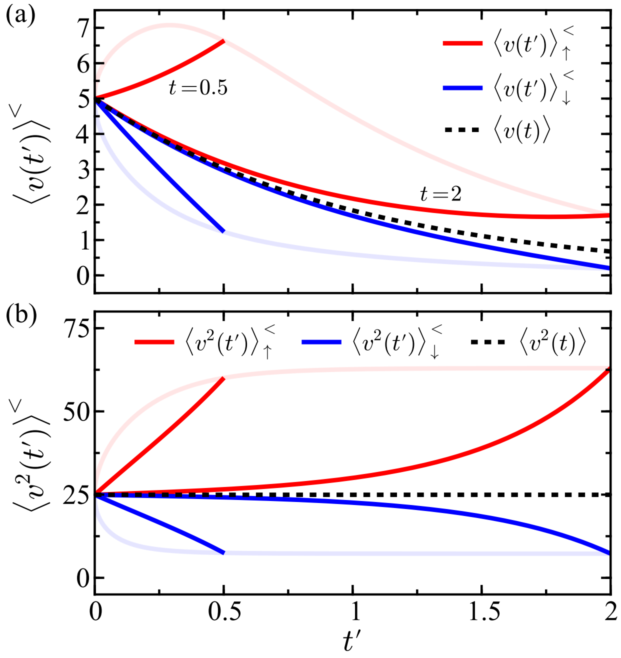


FIG. S5. Two-time once-restricted velocity moments (a) $\langle v(t')\rangle^<$ and (b) $\langle v^2(t')\rangle^<$ as a function of $t'$ for $t = 0.5$ and $t = 2$ and an initial distribution $\delta(v - v_0)$ with $v_0 = \sqrt{\langle v^2\rangle}$. The light transparent curves (red; upside and blue; downside) are the restricted results for $t' = t$ (equivalent curves are shown in Fig. S4). The dashed black curves correspond to the respective unrestricted moment. In both panels the threshold energy is $E^\ddagger = E(0)$.

### D. Two-time Restricted Velocity Moments

For threshold $E^\ddagger = E(0)$ and initial distribution $\rho_0 = \delta(v-v_0)$, the first two-time once-restricted velocity moments are

$$\Big\langle v'\big(t'\big|\, E(t) > E(0),\, v_0\, 0\big)\Big\rangle^<_\uparrow = \langle v(t')\rangle + \sigma_v^2(t')e^{-\gamma(t-t')}\left[\frac{\rho\big(|v_0|\,t\,\big|\,v_0\,0\big) - \rho\big(-|v_0|\,t\,\big|\,v_0\,0\big)}{1-\Phi\big(|v_0|, v_0; t\big) + \Phi\big(-|v_0|, v_0; t\big)}\right] \tag{S47}$$

$$\Big\langle v'\big(t'\big|\, E(t) < E(0),\, v_0\, 0\big)\Big\rangle^<_\downarrow = \langle v(t')\rangle - \sigma_v^2(t')e^{-\gamma(t-t')}\left[\frac{\rho\big(|v_0|\,t\,\big|\,v_0\,0\big) - \rho\big(-|v_0|\,t\,\big|\,v_0\,0\big)}{\Phi\big(|v_0|, v_0; t\big) - \Phi\big(-|v_0|, v_0; t\big)}\right], \tag{S48}$$

and the corresponding second moments are

$$\begin{aligned}\Big\langle v'^2\big(t'\big|\,E(t)>E(0),\,v_0\,0\big)\Big\rangle_{\uparrow}^{<} &= \sigma_v^2(t')+\big\langle v(t')\big\rangle^2\\ &- 2\sigma_v^2(t')\Bigg(v_0e^{-\gamma t}\left[\frac{\sigma_v^2(-t')}{\sigma_v^2(-t)}+\frac{\sigma_v^2(t-t')}{\sigma_v^2(t)}\right]\\ &\quad\times\left[\frac{\rho\big(-|v_0|\,t\,|\,v_0\,0\big)-\rho\big(|v_0|\,t\,|\,v_0\,0\big)}{1-\Phi\big(|v_0|,v_0;t\big)+\Phi\big(-|v_0|,v_0;t\big)}\right]\\ &- |v_0|e^{-2\gamma(t-t')}\frac{\sigma_v^2(t')}{2\sigma_v^2(t)}\\ &\quad\times\left[\frac{\rho\big(-|v_0|\,t\,|\,v_0\,0\big)+\rho\big(|v_0|\,t\,|\,v_0\,0\big)}{1-\Phi\big(|v_0|,v_0;t\big)+\Phi\big(-|v_0|,v_0;t\big)}\right]\Bigg), \qquad \text{(S49)}\\ \Big\langle v'^2\big(t'\big|\,E(t)<E(0),\,v_0\,0\big)\Big\rangle_{\downarrow}^{<} &= \sigma_v^2(t')+\big\langle v(t')\big\rangle^2\\ &+ 2\sigma_v^2(t')\Bigg(v_0e^{-\gamma t}\left[\frac{\sigma_v^2(-t')}{\sigma_v^2(-t)}+\frac{\sigma_v^2(t-t')}{\sigma_v^2(t)}\right]\\ &\quad\times\left[\frac{\rho\big(-|v_0|\,t\,|\,v_0\,0\big)-\rho\big(|v_0|\,t\,|\,v_0\,0\big)}{\Phi\big(|v_0|,v_0;t\big)-\Phi\big(-|v_0|,v_0;t\big)}\right]\\ &- |v_0|e^{-2\gamma(t-t')}\frac{\sigma_v^2(t')}{2\sigma_v^2(t)}\\ &\quad\times\left[\frac{\rho\big(-|v_0|\,t\,|\,v_0\,0\big)+\rho\big(|v_0|\,t\,|\,v_0\,0\big)}{\Phi\big(|v_0|,v_0;t\big)-\Phi\big(-|v_0|,v_0;t\big)}\right]\Bigg). \qquad \text{(S50)}\end{aligned}$$

The dependence of these moments on $t'$ for different $t$ values is shown in Fig. S5. In the limit $t'\to t$, $\langle v(t')\rangle_{\uparrow}^{<}$ and $\langle v(t')\rangle_{\downarrow}^{<}$ respectively approach $\langle v(t)\rangle_{\uparrow}$ and $\langle v(t)\rangle_{\downarrow}$ which are shown as transparent curves (equivalent curves are shown in Fig. S4). In the opposite $t'\to 0$ limit, $\langle v(t')\rangle_{\uparrow}^{<}=\langle v(t')\rangle_{\downarrow}^{<}\to v_0$. Analogous trends are observed in Fig. S5(b) for the second moments, namely, at $t=0$, $\langle v^2(t')\rangle_{\downarrow}^{<}=\langle v^2(t')\rangle_{\downarrow}^{<}=v_0^2$, and for $t'=t$, $\langle v^2(t')\rangle_{\uparrow}^{<}=\langle v^2(t)\rangle_{\uparrow}$ and $\langle v^2(t')\rangle_{\downarrow}^{<}=\langle v^2(t)\rangle_{\downarrow}$. Note that the functional forms of both moments with respect to variation of $t'$ is highly dependent on the specific value of $v_0$.

The expected change in energy over time interval $[0,t]$ for upside and downside processes are:

$$\begin{aligned}\Big\langle \Delta E\big(t\,\big|\,E(t)>E(0),v_0\,0\big)\Big\rangle_{\uparrow} &= \int_{\mathbb{R}}\big[E(v)-E(0)\big]\tilde{\rho}_{\uparrow}(v\,t\,|\,v_0\,0)\,dv\\ &= \frac{1}{2}m\Big\langle v^2\big(t\,\big|\,E(t)>E(0),v_0\,0\big)\Big\rangle_{\uparrow}-E(0), \qquad \text{(S51)}\\ \Big\langle \Delta E\big(t\,\big|\,E(t)<E(0),v_0\,0\big)\Big\rangle_{\downarrow} &= \int_{\mathbb{R}}\big[E(v)-E(0)\big]\tilde{\rho}_{\downarrow}(v\,t\,|\,v_0\,0)\,dv\\ &= \frac{1}{2}m\Big\langle v^2\big(t\,\big|\,E(t)>E(0),v_0\,0\big)\Big\rangle_{\downarrow}-E(0). \qquad \text{(S52)}\end{aligned}$$

where the respective restricted second velocity moments can be taken directly from Eqs. (S43) and (S44). In this case $\langle \Delta E \rangle$ is given by the difference between the energy of the respective restricted process at time $t$ and the initial energy $E_0$ at time $t' = 0$, which is the same for every trajectory in the ensemble.

### E. Velocity Correlation Function

For threshold $E^{\ddagger} = E(0)$ and an initial $\delta$-distribution, the restricted velocity correlation functions are:

$$\begin{aligned} \big\langle v'(t')v(t) \big| \, E(t) > E(0), \, v_0 \, 0 \big\rangle_{\uparrow}^{<} &= e^{-\gamma(t-t')} \Big( \sigma_v^2(t') + \big\langle v(t') \big\rangle^2 \Big) - 2 \big\langle v(t') \big\rangle \sigma_v^2(t) \\ &\quad \times \left[ \frac{\rho\big( -|v_0| \, t \, \big| \, v_0 \, 0 \big) - \rho\big( |v_0| \, t \, \big| \, v_0 \, 0 \big)}{1 - \Phi\big( |v_0|, v_0; t \big) + \Phi\big( -|v_0|, v_0; t \big)} \right] \\ &\quad + 2|v_0| e^{-\gamma(t-t')} \sigma_v^2(t') \\ &\quad \times \left[ \frac{\rho\big( -|v_0| \, t \, \big| \, v_0 \, 0 \big) + \rho\big( |v_0| \, t \, \big| \, v_0 \, 0 \big)}{1 - \Phi\big( |v_0|, v_0; t \big) + \Phi\big( -|v_0|, v_0; t \big)} \right], \end{aligned} \tag{S53}$$

$$\begin{aligned} \big\langle v'(t')v(t) \big| \, E(t) < E(0), \, v_0 \, 0 \big\rangle_{\downarrow}^{<} &= e^{-\gamma(t-t')} \Big( \sigma_v^2(t') + \big\langle v(t') \big\rangle^2 \Big) + 2 \big\langle v(t') \big\rangle \sigma_v^2(t) \\ &\quad \times \left[ \frac{\rho\big( -|v_0| \, t \, \big| \, v_0 \, 0 \big) - \rho\big( |v_0| \, t \, \big| \, v_0 \, 0 \big)}{\Phi\big( |v_0|, v_0; t \big) - \Phi\big( -|v_0|, v_0; t \big)} \right] \\ &\quad - 2|v_0| e^{-\gamma(t-t')} \sigma_v^2(t') \\ &\quad \times \left[ \frac{\rho\big( -|v_0| \, t \, \big| \, v_0 \, 0 \big) + \rho\big( |v_0| \, t \, \big| \, v_0 \, 0 \big)}{\Phi\big( |v_0|, v_0; t \big) - \Phi\big( -|v_0|, v_0; t \big)} \right]. \end{aligned} \tag{S54}$$

---


[1] E. W. Ng and M. Geller, Journal of Research of the National Bureau of Standards B **73**, 120 (1969).

[2] M. K. Simon and D. Divsalar, IEEE Trans. Commun. **46**, 200 (1998), doi:10.1109/26.659479.

[3] H. Fayed and A. Atiya, Math. Comp **83**, 235 (2014), doi:10.1090/S0025-5718-2013-02720-2.

[4] H. Fayed, A. Atiya, and A. Badawi, Math. Sci. Lett. **4**, 249 (2015), doi:10.12785/msl/040305.
